# Supplementary material for: Exploring Post-Training Quantization of Protein Language Models
Source: arXiv:2310.19624 source file (2023-10-30)
Supplement: Supplementary file 1 [file appendix.tex]

\subsection{Methodology Details}
\paragraph{Clipping Strategies}
There are two main strategies to determine the clipping range for activation quantization. We sort the activation values from smallest to largest and use the following methods to select the clipping range $[r_l, r_u]$.

\begin{itemize}
 \item Average: This approach identifies the upper and lower bounds of the clipping range by taking the average of the Top-$k$ maximum and minimum activation values.
 \item Median: This approach identifies the upper and lower bounds of the clipping range by using the median of the Top-$k$ maximum and minimum activation values.
\end{itemize}

Experimental results indicate that the \textsl{Median} strategy performs better than the \textsl{Average} strategy. Therefore, in this paper, we adopt the \textsl{Median} strategy to determine the clipping range.

\paragraph{Explanations of Equation (6)}
We assume that the distribution of activations follows a Gaussian distribution. In this case, finding the optimal breakpoints can be achieved through gradient descent, as this is a convex optimization problem. However, the gradient descent method for calculating the optimal breakpoints is slow. We take a faster approximation using $p = \ln(m\cdot r + n)$ for normalized Gaussian to address this issue.
Experimental results demonstrate that this approximation achieves nearly the same level of accuracy as the gradient descent method while being considerably faster in computation. As a result, we utilize this approximated version of the optimal breakpoints in this paper.

\subsection{Additional Experiment Details}
\paragraph{Size of Calibration Datasets}
The size of calibration data has a direct impact on the issue of data accessibility in post-training quantization. To investigate its effects, we varied the calibration data size from 16 to 128. We observed that the prediction score of PTQ4Protein gradually increases and then saturates after 100 calibration data samples, as shown in Table~\ref{appendix_v1}. Based on this observation, we hypothesize that PTQ4Protein does not require a larger number of training instances for optimization.
Since we found diminishing gains in increasing the calibration data size beyond 100 samples, we default to using 100 samples for calibration in our experiments.

\paragraph{Different Clipping Strategies and Ranges}
We present our experimental findings for various strategies and ranges in Table~\ref{appendix_v2}. Overall, the \textsl{Median} strategy performs better than the \textsl{Average} strategy, indicating that the distribution of activation values is highly imbalanced. Thus, the \textsl{Average} strategy may result in inaccurate clipping ranges. Additionally, we observed that as the clipping range decreases, the prediction score of PTQ4Protein also decreases gradually. This suggests that a wider clipping range is more suitable for the activation quantization of ESMFold.

\begin{table*}
    \centering
    \begin{tabular}{c|c|cc}
        \toprule
         Quantization Mode & Calibration Data Size & CASP14 & CAMEO \\
         \midrule
         \multirow{5}{*}{W8A8} & 16 & 48.11 & 71.52 \\
         & 32 & 48.16 & 71.80 \\
         & 64 & 49.03 & 72.32 \\
         & 100 & 49.87 & 73.43 \\
         & 128 & 49.88 & 73.43 \\
         \bottomrule
    \end{tabular}
    \caption{Evaluation results of ESMFold's activation quantization with varying calibration dataset sizes.}
    \label{appendix_v1}
\end{table*}

\begin{table*}
\centering
\begin{tabular}{l|c|cc}
\toprule
Clipping Strategies & Clipping Ranges & CASP14 & CAMEO \\ 
\midrule
\multirow{3}{*}{Average (W8A8)} & Top-1 & 49.85 & 73.18 \\ 
 & Top-5 & 49.76 & 73.11 \\ 
 & Top-30 & 47.95 & 71.60  \\ 
 & Top-100 & 47.08 & 70.99  \\ 
 \midrule
\multirow{3}{*}{Median (W8A8)} & Top-1 & 49.65 & 73.21  \\ 
 & Top-5 &  49.87 & 73.43 \\ 
 & Top-30 & 48.01 & 72.35 \\ 
 & Top-100 & 47.66 & 71.92 \\ 
 \midrule
\end{tabular}
\caption{Evaluation results of activation quantization for ESMFold with varied clipping strategies and ranges.}
\label{appendix_v2}
\end{table*}
